# Supplementary material for: Local finiteness for real-virtual corrections to electroweak production in partonic collisions
Source: arXiv:2601.22936 source file (2026-01-30)

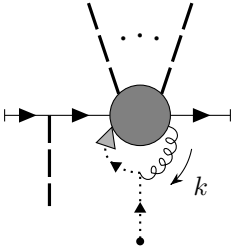

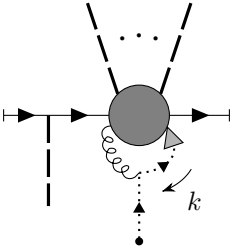

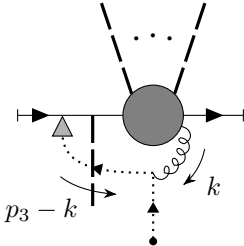

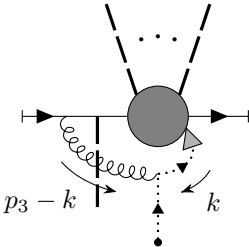

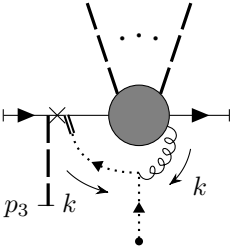

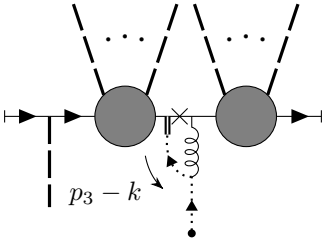

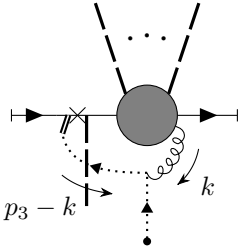

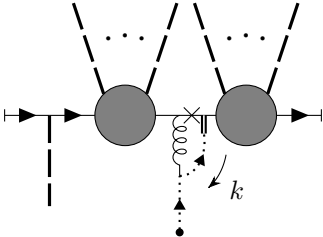



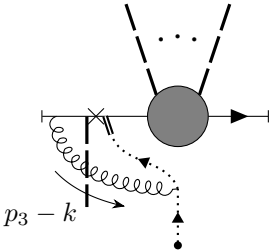

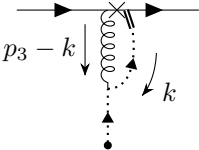

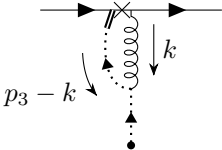

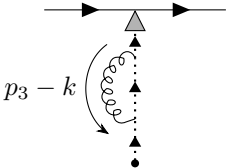

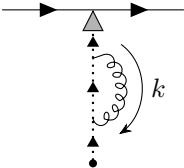

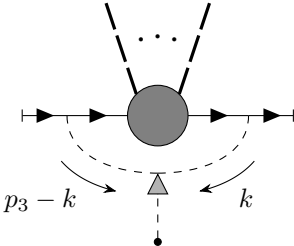

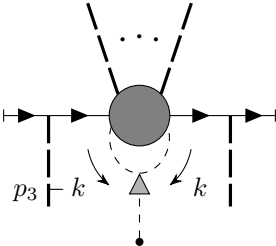

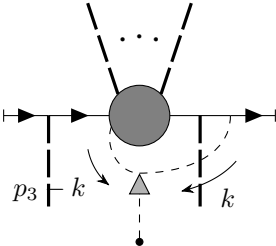



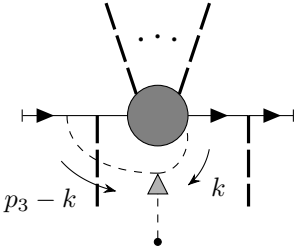

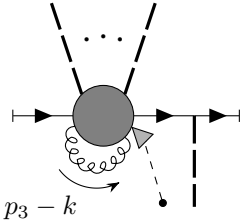

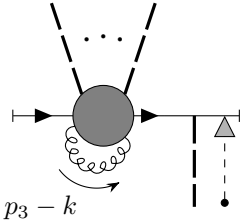

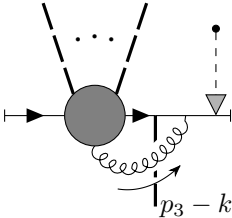

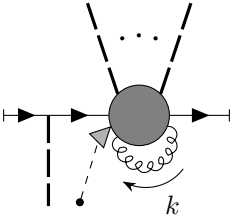

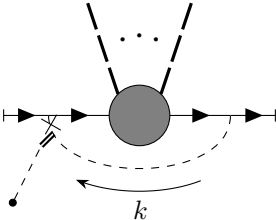

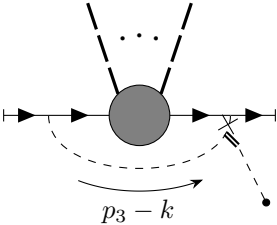

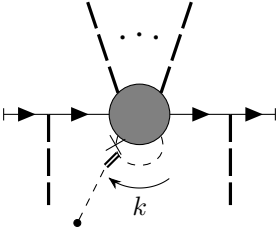



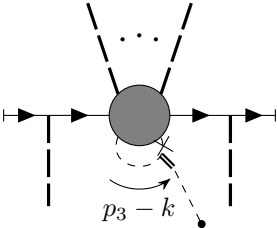

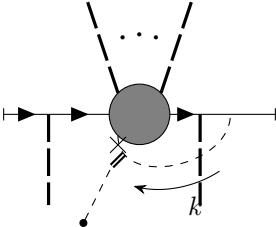

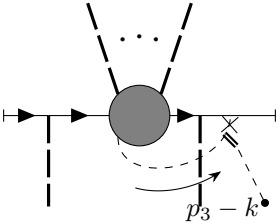

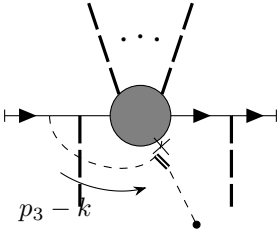

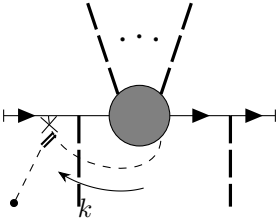

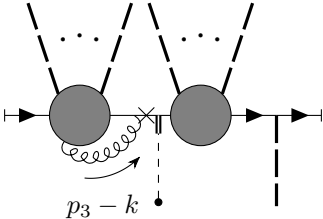

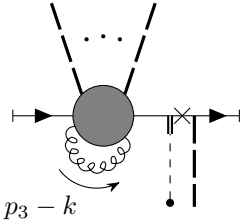

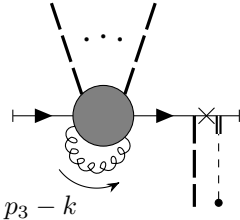



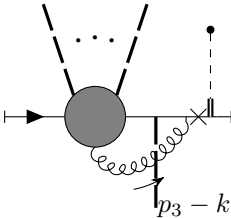

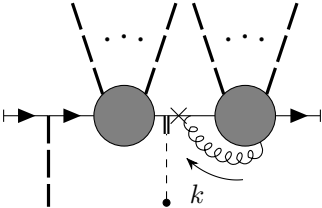

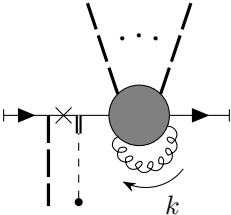

Supplement: Supplementary file 1 [file tikz_RV_blob_appendix_LC.pdf]
