# Supplementary material for: Local finiteness for real-virtual corrections to electroweak production in partonic collisions
Source: arXiv:2601.22936 source file (2026-01-30)

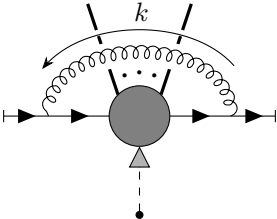

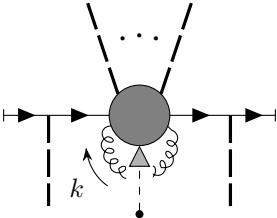

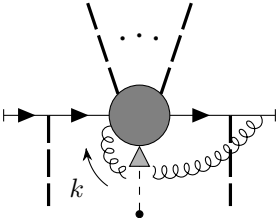

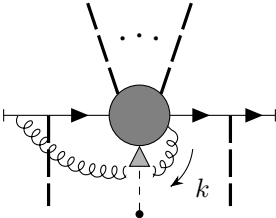

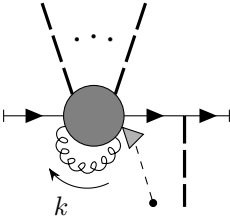

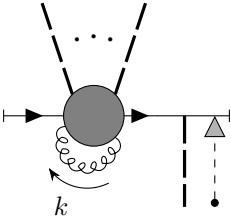

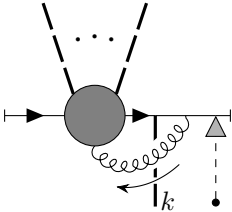

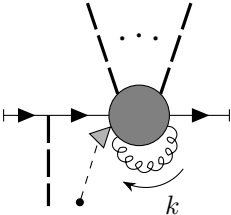



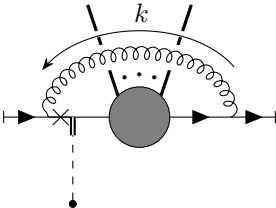

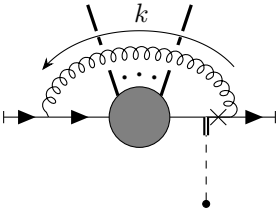

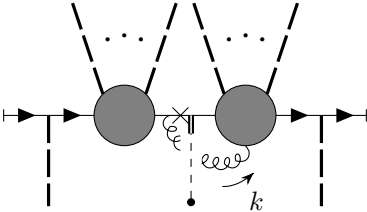

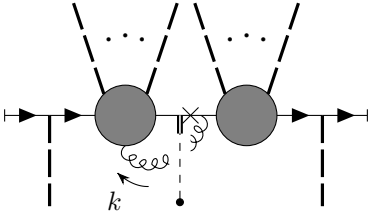

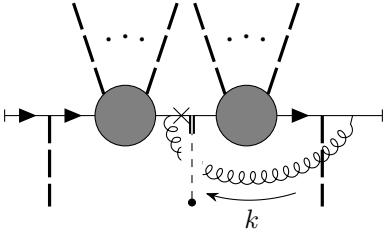

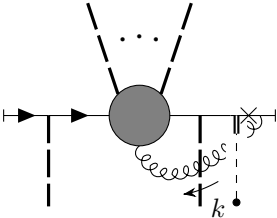

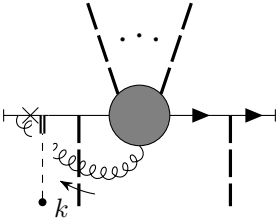

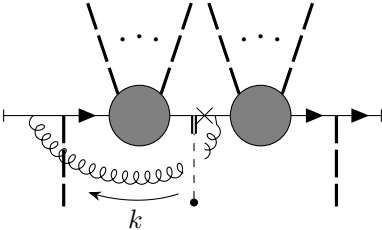



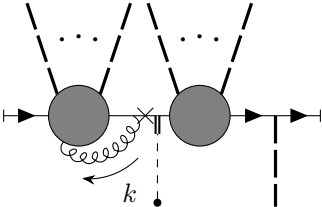

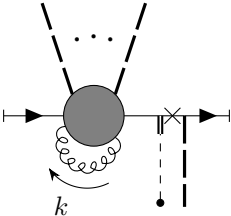

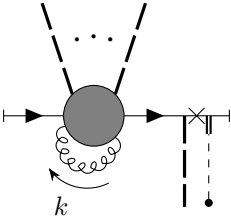

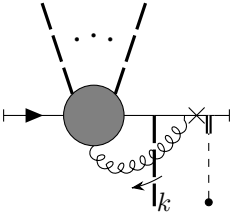

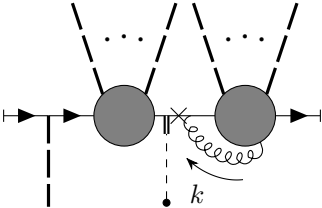

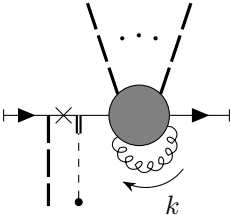

Supplement: Supplementary file 2 [file tikz_RV_blob_appendix_SLC.pdf]
